# Supplementary material for: Interoceptive Divergence in Aesthetic Evaluation and Implications for Human-AI Alignment
Source: arXiv:2605.18759 source file (2026-04-05)
Supplement: Supplementary file 1 [file supplementary.tex]

In this section, we provide detailed examples of the prompts used in the experiments as well as the results of additional analyses. 
In the supplementary analyses, we examined the relationships between valence, arousal, and emotion labels for both humans and AI. 
In addition, we investigated the relationship between personality traits and the strength of responses to image features. 
Furthermore, we examined the co-occurrence of sadness and beauty--so-called "sad beauty"--in both humans and AI.

\clearpage
\subsection{Prompts for Aesthetic Evaluation} 

The prompts used for this study are as follows\footnote{
Regarding the method for eliciting body map responses, alternative phrasings such as "When you see the image, which parts of your body do you feel sensations in?" or "Can you imagine specific body parts corresponding to the sensations triggered by this image?" were also considered. 
However, such formulations frequently resulted in cases where LLMs, lacking a physical body, did not provide body map responses. 
Therefore, the current prompt formulation was adopted. 
A similar issue has been reported in prior work by Xu et al.~\citep{xu2025largelanguagemodelssensorimotor}, where LLMs refused to respond on the grounds that they do not possess a body, and prompt adjustments were introduced as a countermeasure. 
}.

\vspace{0.5cm}
\textbf{System Prompt}

\begin{quotation}
    \texttt{\normalsize{
You will be asked to answer to questions about the image that will be presented to you.
When answering, output only in JSON format. Refrain from outputting anything other than JSON format.
}}
\end{quotation}

\textbf{System Prompt (Japanese)} 
\begin{quotation}
    \texttt{\normalsize{
あなたは，提示される画像に関する質問に答えるよう求められます．
回答する際は，JSON形式のみで出力してください．JSON形式以外の出力は控えてください．
}}
\end{quotation}

\textbf{User Prompt}
\begin{quotation}
    \texttt{\normalsize{
Q1:
Which body parts do you feel are most associated with the image?
The list of body parts is: head, upper abdomen, lower abdomen, right hand, left hand, right foot, and left foot.
For each part where you feel an association, enter an integer greater than 0.
If the association is strong, provide a larger number.
\\
Q2:
Please rate the difficulty of the previous task (Q1) on a scale from 1 (easy) to 9 (difficult).
\\
Q3: 
Please rate your impression of the presented image on a 9-point scale.
Valence (1 = unpleasant/negative, 9 = pleasant/positive)
Arousal (1 = calm/relaxed, 9 = excited)
Beauty (1 = ugly/not beautiful at all, 9 = very beautiful)
}}
\end{quotation}

% \vspace{1cm}
\textbf{Ranking Method}
\begin{quotation}
    \texttt{\normalsize{
Q4: 
Please rank the emotions you feel from the presented image by selecting top three different items.
You cannot select the same item for different ranks.
Here are the emotion options: Admiration, Adoration, Amusement, Anger, Anxiety, Awe, Awkwardness, Boredom, Calmness, Confusion, Contempt, Craving, Disappointment, Disgust, Empathic pain, Entrancement, Envy, Excitement, Fear/Horror, Guilt, Interest, Joy, Nostalgia, Pride, Relief, Romance, Sadness, Satisfaction, Sexual desire, Surprise, Sympathy, Triumph
\\
Note: \\
- Answer in English.\\
- Ensure that your output is strictly in JSON format without any additional characters or formatting symbols such as ``` before and after the JSON object.\\
- Strictly adhere to the example format provided below:\\
\{
    "Q1-head": 0, 
    "Q1-upper-abdomen": 0,
    "Q1-lower-abdomen": 1,
    "Q1-right-hand": 2,
    "Q1-left-hand": 0,
    "Q1-right-foot": 0,
    "Q1-left-foot": 5,
    "Q2-difficulty": 6,
    "Q3-valence": 2, 
    "Q3-arousal": 9,
    "Q3-beauty": 4,
    "Q4-top1": "Anger",
    "Q4-top2": "Boredom",
    "Q4-top3": "Triumph",
\}
}}
\end{quotation}

\textbf{Rating Method}
\begin{quotation}
    \texttt{\normalsize{
Q4: 
Please rate the intensity of each of the following emotions you feel from the presented image using a 9-point Likert scale (1 = very weak, 9 = very strong).
You must provide a numeric value from 1 to 9 for each emotion, based on how strongly you experienced that emotion when viewing the image.
\\
Here are the emotion options: Admiration, Adoration, Amusement, Anger, Anxiety, Awe, Awkwardness, Boredom, Calmness, Confusion, Contempt, Craving, Disappointment, Disgust, Empathic pain, Entrancement, Envy, Excitement, Fear/Horror, Guilt, Interest, Joy, Nostalgia, Pride, Relief, Romance, Sadness, Satisfaction, Sexual desire, Surprise, Sympathy, Triumph
\\
Note: \\
- Answer in English.\\
- Ensure that your output is strictly in JSON format without any additional characters or formatting symbols such as ``` before and after the JSON object.\\
- Strictly adhere to the example format provided below:\\
\{
    "Q1-head": 0, 
    "Q1-upper-abdomen": 0,
    "Q1-lower-abdomen": 1,
    "Q1-right-hand": 2,
    "Q1-left-hand": 0,
    "Q1-right-foot": 0,
    "Q1-left-foot": 5,
    "Q2-difficulty": 6,
    "Q3-valence": 2, 
    "Q3-arousal": 9,
    "Q3-beauty": 4,
    "Q4-Admiration": 3,
    "Q4-Adoration": 1,
    "Q4-Amusement": 5,
    "Q4-Anger": 2,
    "Q4-Anxiety": 4,
    "Q4-Awe": 6,
    "Q4-Awkwardness": 1,
    "Q4-Boredom": 2,
    "Q4-Calmness": 7,
    "Q4-Confusion": 3,
    "Q4-Contempt": 1,
    "Q4-Craving": 5, 
    "Q4-Disappointment": 2,
    "Q4-Disgust": 1,
    "Q4-Empathic pain": 4,
    "Q4-Entrancement": 6,
    "Q4-Envy": 1,
    "Q4-Excitement": 8,
    "Q4-Fear/Horror": 2,
    "Q4-Guilt": 3,
    "Q4-Interest": 7,
    "Q4-Joy": 6,
    "Q4-Nostalgia": 5,
    "Q4-Pride": 4,
    "Q4-Relief": 3,
    "Q4-Romance": 1,
    "Q4-Sadness": 2,
    "Q4-Satisfaction": 5,
    "Q4-Sexual desire": 2,
    "Q4-Surprise": 6,
    "Q4-Sympathy": 3,
    "Q4-Triumph": 7,
\}
}}
\end{quotation}

\textbf{User Prompt (Japanese)} 
\begin{quotation}
    \texttt{\normalsize{
Q1:
この画像に最も関連していると感じる身体の部位はどれですか？
身体の部位のリストは，頭，上腹部，下腹部，右手，左手，右足，左足です．
関連性を感じる部位には，0より大きい整数を入力してください．
関連性が強い場合は，より大きな数を入力してください．
\\
Q2:
前のタスク（Q1）の難易度（1:簡単，9:難しい）をお答えください．
\\
Q3:
提示された画像に対するイメージ（印象）について，9段階で回答してください．
感情価（1 = 不快/ネガティブ，9 = 快適/ポジティブ）
覚醒度（1 = 穏やか/落ち着き，9 = 興奮）
美しさ（1 = 醜い/まったく美しくない，9 = とても美しい）
}}
\end{quotation}

\textbf{Ranking Method}
\begin{quotation}
    \texttt{\normalsize{
Q4:
提示された画像から感じる感情を，トップ3の異なる項目を選択してランク付けしてください．
異なるランクに同じ項目を選択することはできません．
感情の選択肢は以下の通りです：
'称賛，憧れ', '崇拝', '娯楽的な楽しみ', '怒り', '不安', '畏怖，畏敬（いふ，いけい）',
'ぎこちなさ，不自然さ', '退屈', '静けさ', '困惑', '軽蔑', '切望', '失望感', '嫌悪感', '共感',
'狂喜，有頂天', 'ねたみ', '興奮', '恐れ', '罪悪感', '興味', '喜び，うれしさ', '懐かしさ，郷愁',
'プライド，誇り', '安心', 'ロマンス', '悲しみ', '満足，充足', '性欲', '驚き', '同情', '勝利，征服'
\\
注意:\\
- 日本語で回答してください．\\
- 出力はJSON形式で，追加の文字やフォーマット記号（例：```）は使用しないでください．\\
- 以下の例の形式に厳密に従ってください：\\
\{
    "Q1-頭": 0, 
    "Q1-上腹部": 0,
    "Q1-下腹部": 1,
    "Q1-右手": 2,
    "Q1-左手": 0,
    "Q1-右足": 0,
    "Q1-左足": 5,
    "Q2-難易度": 6,
    "Q3-感情価": 2, 
    "Q3-覚醒度": 9,
    "Q3-美しさ": 4,
    "Q4-トップ1": "怒り",
    "Q4-トップ2": "退屈",
    "Q4-トップ3": "勝利，征服",
\}
}}
\end{quotation}

\textbf{Rating Method}
\begin{quotation}
    \texttt{\normalsize{
Q4:
提示された画像から感じる各感情の強度を，9段階のリッカート尺度（1 = 非常に弱い，9 = 非常に強い）を使用して評価してください．
各感情について，画像を見たときにその感情をどれだけ強く感じたかに基づいて，1から9の数値を回答する必要があります．
感情の選択肢は以下の通りです：
'称賛，憧れ', '崇拝', '娯楽的な楽しみ', '怒り', '不安', '畏怖，畏敬（いふ，いけい）',
'ぎこちなさ，不自然さ', '退屈', '静けさ', '困惑', '軽蔑', '切望', '失望感', '嫌悪感', '共感',
'狂喜，有頂天', 'ねたみ', '興奮', '恐れ', '罪悪感', '興味', '喜び，うれしさ', '懐かしさ，郷愁',
'プライド，誇り', '安心', 'ロマンス', '悲しみ', '満足，充足', '性欲', '驚き', '同情', '勝利，征服'
\\
注意:\\
- 日本語で回答してください．\\
- 出力はJSON形式で，追加の文字やフォーマット記号（例：```）は使用しないでください．\\
- 以下の例の形式に厳密に従ってください：\\
\{
    "Q1-頭": 0, 
    "Q1-上腹部": 0,
    "Q1-下腹部": 1,
    "Q1-右手": 2,
    "Q1-左手": 0,
    "Q1-右足": 0,
    "Q1-左足": 5,
    "Q2-難易度": 6,
    "Q3-感情価": 2, 
    "Q3-覚醒度": 9,
    "Q3-美しさ": 4,
    "Q4-称賛，憧れ": 3,
    "Q4-崇拝": 1,
    "Q4-娯楽的な楽しみ": 5,
    "Q4-怒り": 2,
    "Q4-不安": 4,
    "Q4-畏怖，畏敬（いふ，いけい）": 6,
    "Q4-ぎこちなさ，不自然さ": 1,
    "Q4-退屈": 2,
    "Q4-静けさ": 7,
    "Q4-困惑": 3,
    "Q4-軽蔑": 1,
    "Q4-切望": 5,
    "Q4-失望感": 2,
    "Q4-嫌悪感": 1,
    "Q4-共感": 4,
    "Q4-狂喜，有頂天": 6,
    "Q4-ねたみ": 1,
    "Q4-興奮": 8,
    "Q4-恐れ": 2,
    "Q4-罪悪感": 3,
    "Q4-興味": 7,
    "Q4-喜び，うれしさ": 6,
    "Q4-懐かしさ，郷愁": 5,
    "Q4-プライド，誇り": 4,
    "Q4-安心": 3,
    "Q4-ロマンス": 1,
    "Q4-悲しみ": 2,
    "Q4-満足，充足": 5,
    "Q4-性欲": 2,
    "Q4-驚き": 6,
    "Q4-同情": 3,
    "Q4-勝利，征服": 7,
\}
}}
\end{quotation}

% \clearpage
After obtaining all evaluation responses within a single API call, a subsequent call was made to request explanations for those judgments. 
\vspace{0.5cm}

\textbf{Follow-Up User Prompt for Eliciting Explanations}
\begin{quotation}
    \texttt{\normalsize{
Can you explain the reasoning behind your answers to Q1 through Q4?
In addtion, please describe the content of the image in detail.
\\
Note: \\
- Answer in English.\\
- Ensure that your output is strictly in JSON format without any additional characters or formatting symbols such as ``` before and after the JSON object.\\
- Strictly adhere to the example format provided below:\\
\{
    "Q1-reason": "Because \textasciitilde\textasciitilde\textasciitilde.",     
    "Q2-reason": "Because \textasciitilde\textasciitilde\textasciitilde.", 
    "Q3-reason": "Because \textasciitilde\textasciitilde\textasciitilde.", 
    "Q4-reason": "Because \textasciitilde\textasciitilde\textasciitilde.", 
    "Description": "The image depicts \textasciitilde\textasciitilde\textasciitilde."
\}
}}
\end{quotation}

\textbf{Follow-Up User Prompt for Eliciting Explanations (Japanese)}
\begin{quotation}
    \texttt{\normalsize{
Q1からQ4までの回答の理由を説明できますか？
さらに，画像の内容を詳細に説明してください．
\\
注意:\\
- 日本語で回答してください．\\
- 出力はJSON形式で，追加の文字やフォーマット記号（例：```）は使用しないでください．\\
- 以下の例の形式に厳密に従ってください：\\
\{
    "Q1-理由": "なぜなら，\textasciitilde\textasciitilde\textasciitilde だからです．",
    "Q2-理由": "なぜなら，\textasciitilde\textasciitilde\textasciitilde だからです．",
    "Q3-理由": "なぜなら，\textasciitilde\textasciitilde\textasciitilde だからです．",
    "Q4-理由": "なぜなら，\textasciitilde\textasciitilde\textasciitilde だからです．",
    "説明": "画像は，\textasciitilde\textasciitilde\textasciitilde を描いています．"
\}
}}
\end{quotation}

\clearpage
\subsection{Supplementary Analysis 1: Relationship with Valence and Arousal}
The results of the correlation analysis between valence/arousal scores and emotion intensity scores for each image are shown in Figure~\ref{fig:va_emotion_correlation}. 
Specifically, for both humans and AI, emotions such as Admiration, Amusement, Joy, Relief, and Satisfaction showed strong positive correlations with valence, whereas emotions such as Anxiety, Awkwardness, Confusion, Disappointment, and Disgust showed strong negative correlations with valence. 
In addition, for both humans and AI, emotions such as Amusement, Excitement, and Surprise showed strong positive correlations with arousal, while Calmness showed a strong negative correlation with arousal.

\begin{figure*}[htbp]
  \centering
  \begin{subfigure}[t]{\textwidth}
    \includegraphics[width=\columnwidth, trim=0 0 0 0, clip]{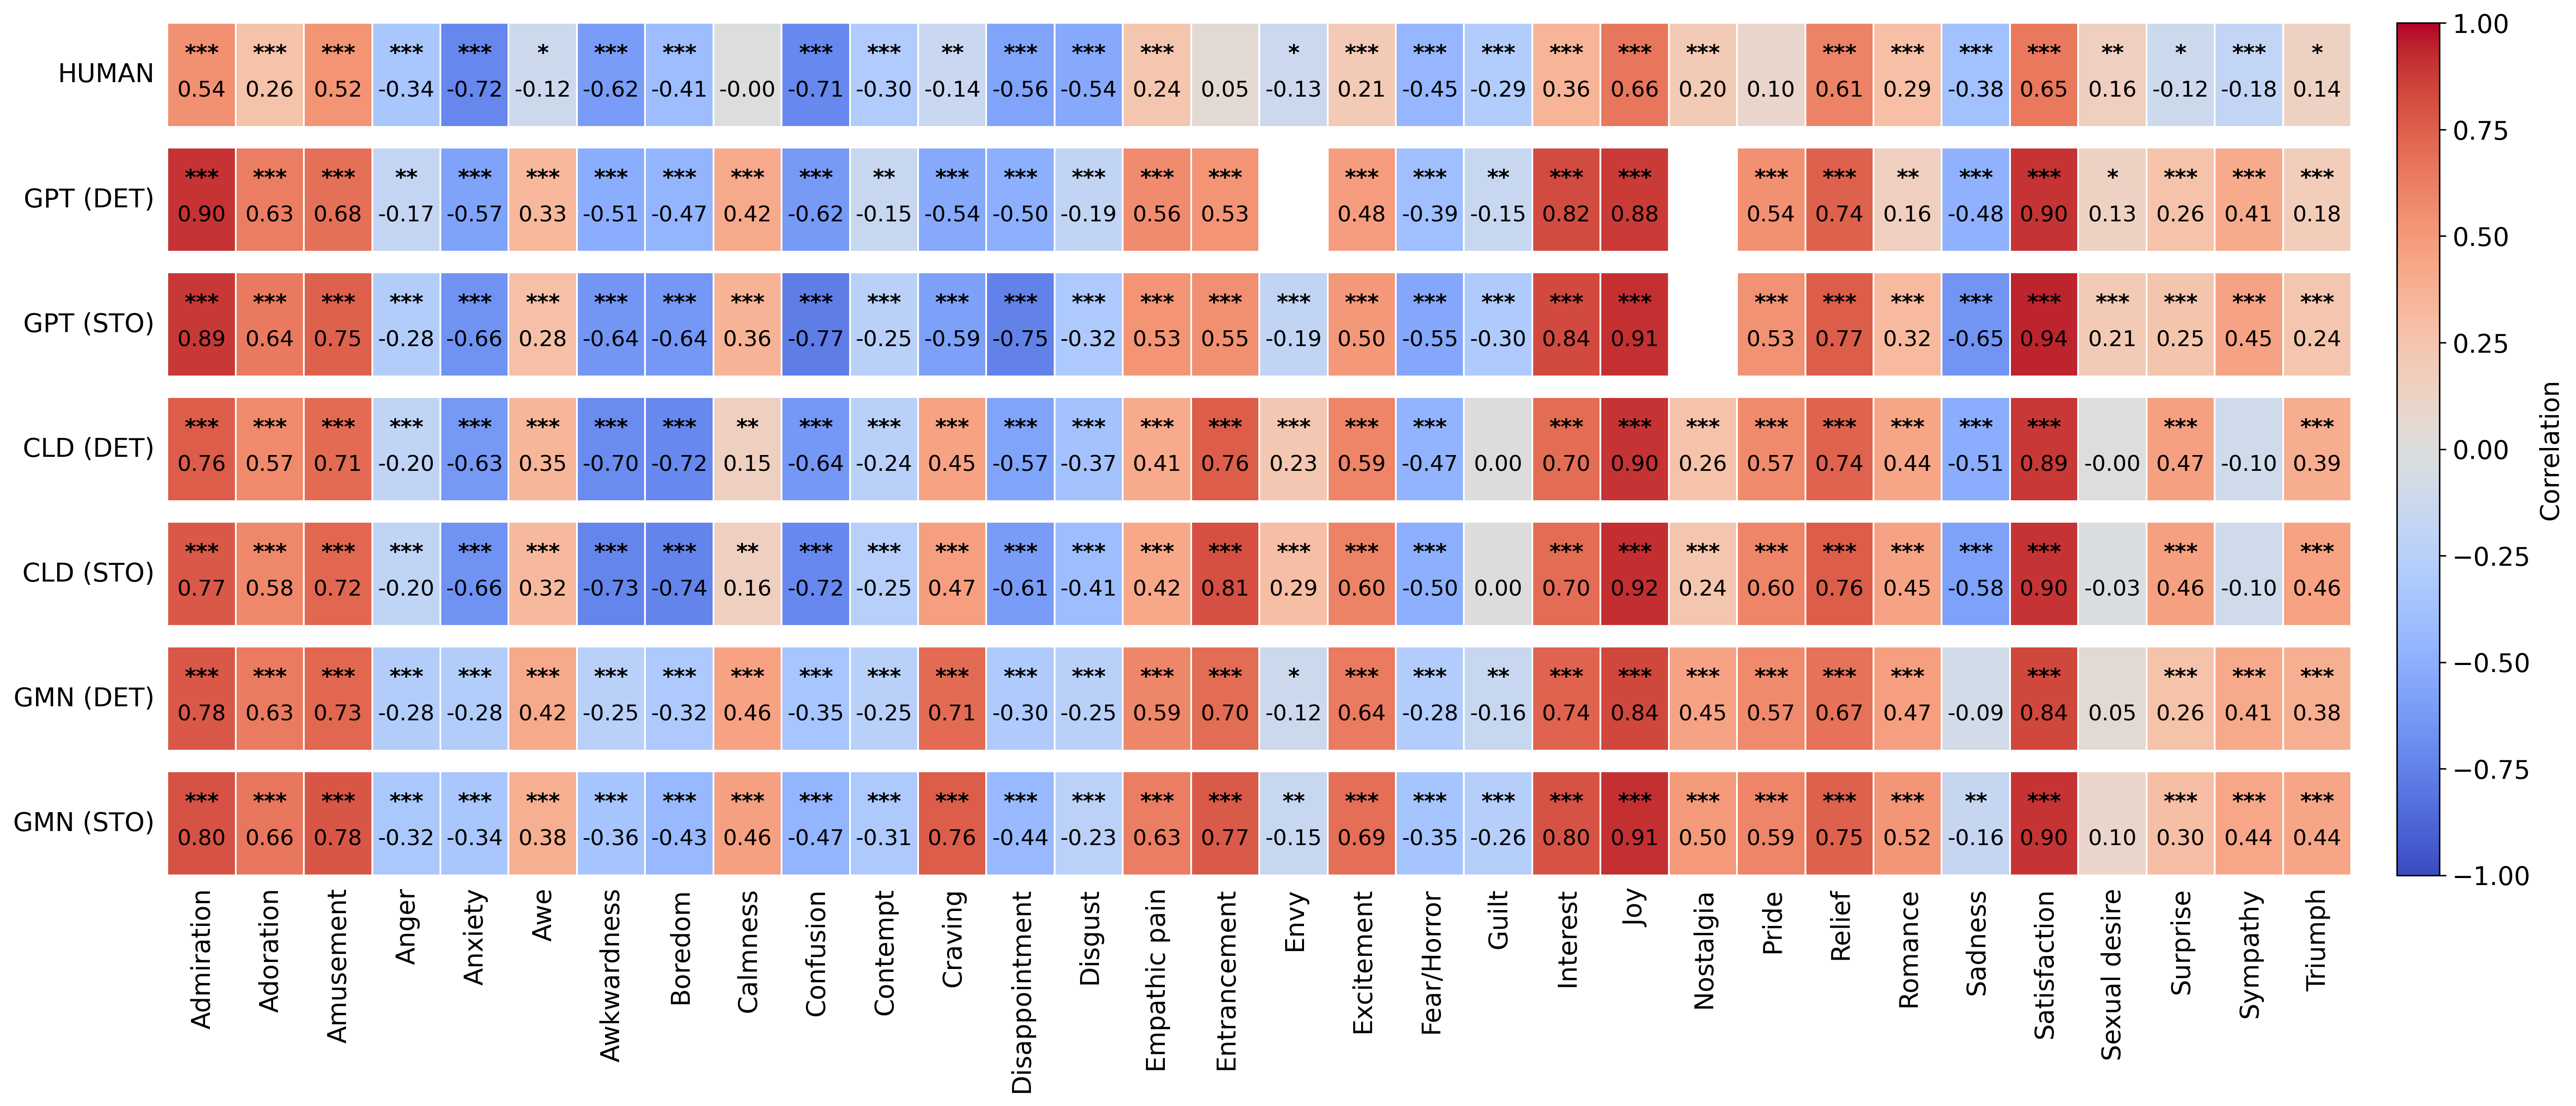}
    % \fbox{\rule{0pt}{4.5cm}\rule{\columnwidth}{0pt}}
    \caption{Correlation between the valence and emotion intensity scores}
  \end{subfigure}\\
  \vspace{7mm}
  \begin{subfigure}[t]{\textwidth}
    \includegraphics[width=\columnwidth, trim=0 0 0 0, clip]{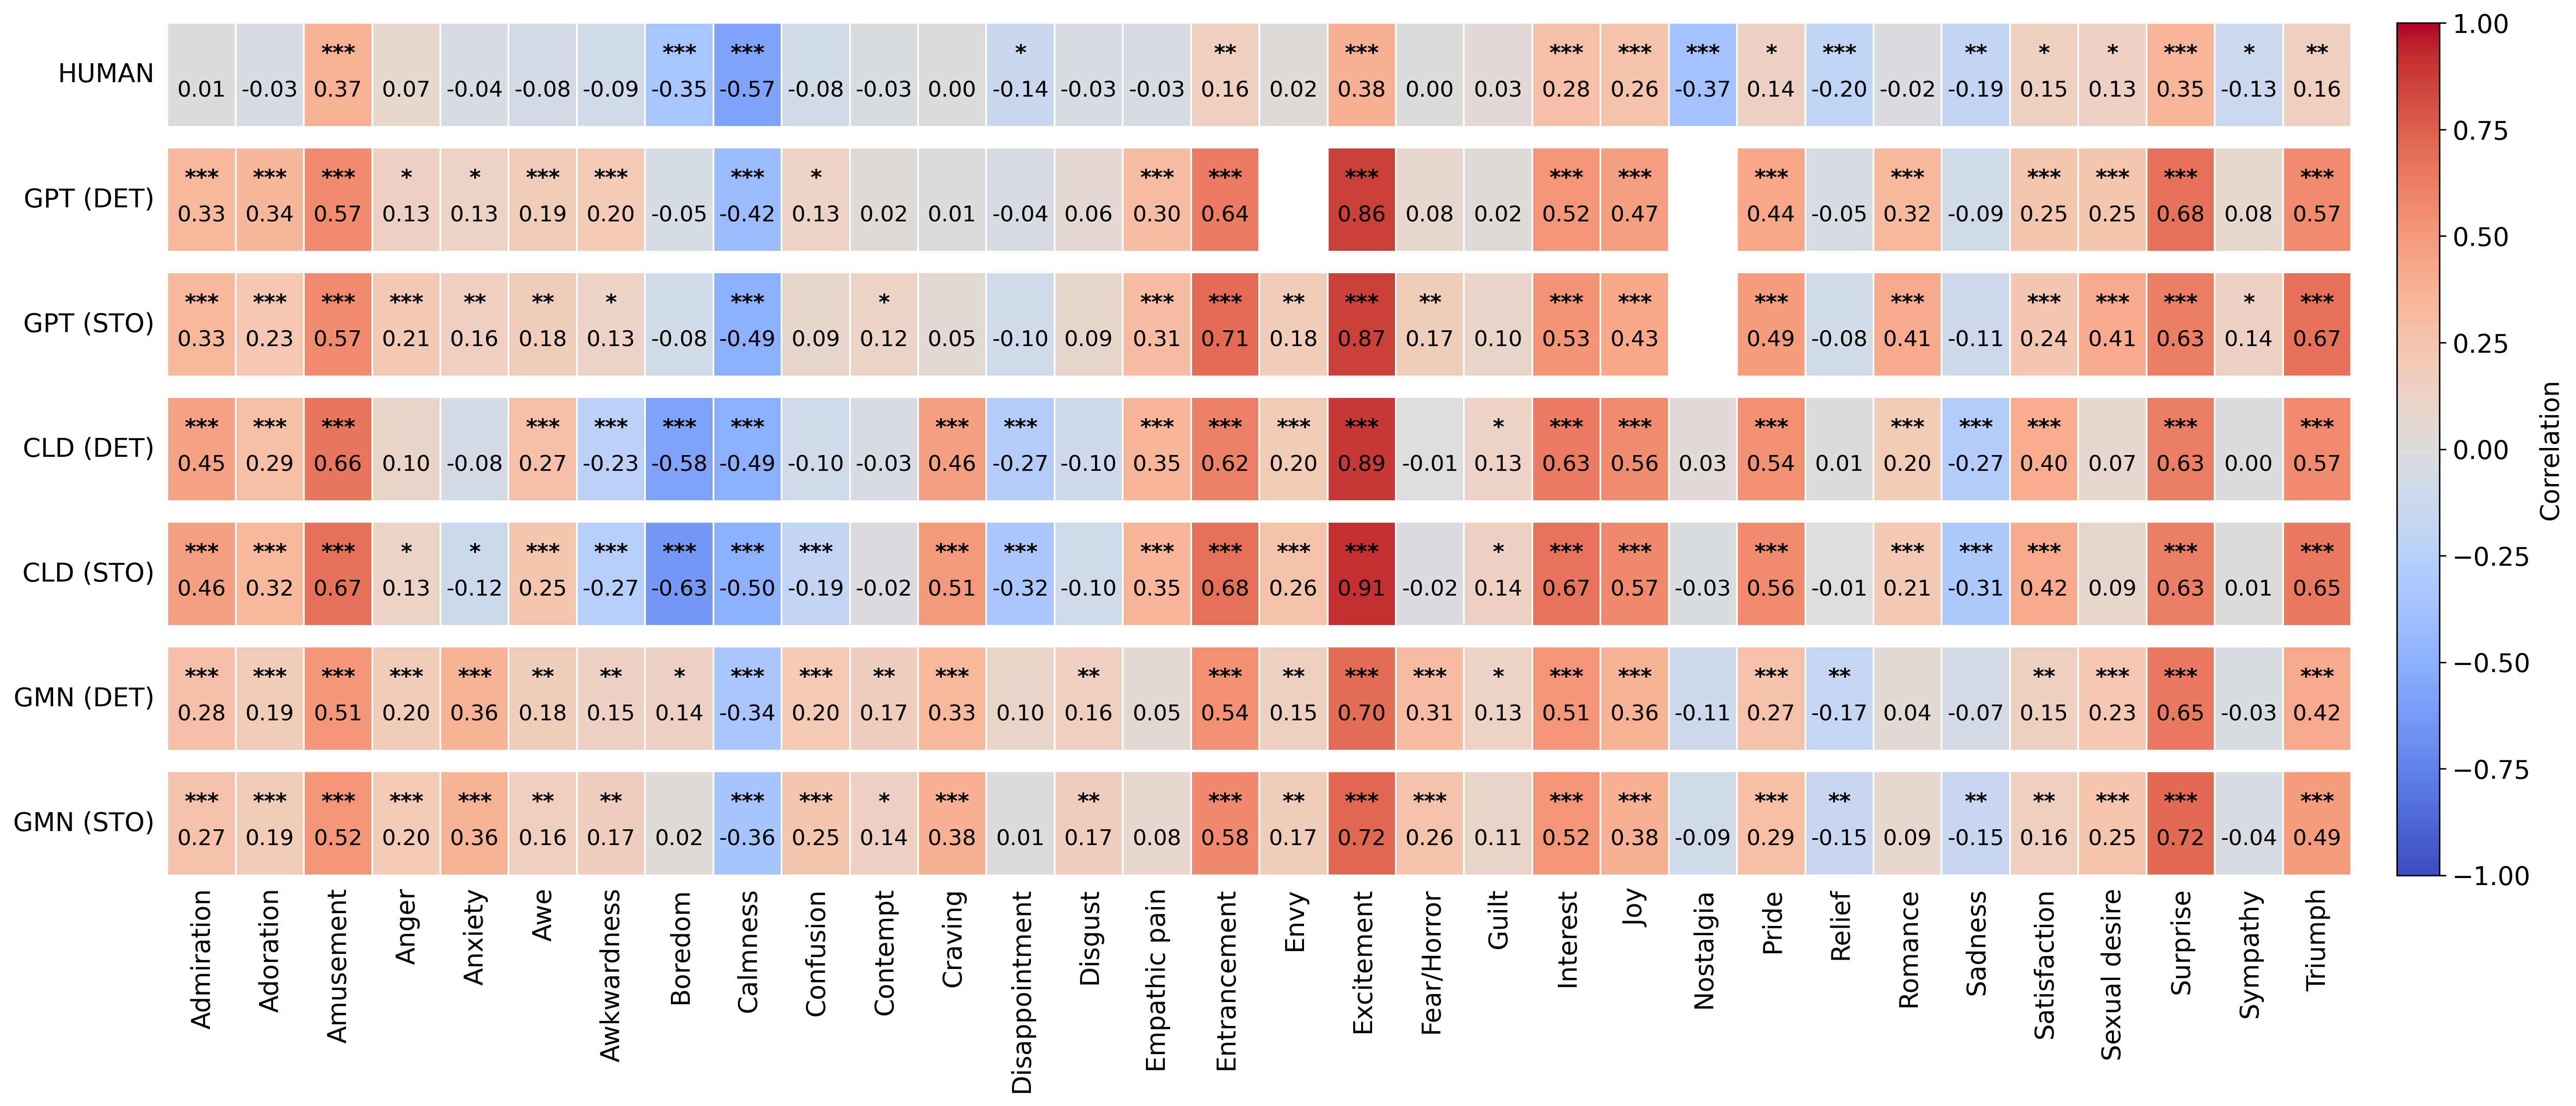}
    % \fbox{\rule{0pt}{4.5cm}\rule{\columnwidth}{0pt}}
    \caption{Correlation between the arousal and emotion intensity scores}
  \end{subfigure}
  % \fbox{\rule{0pt}{4.5cm}\rule{0.45\columnwidth}{0pt}}
  \caption[Spearman's rank correlation coefficients between the valence/arousal and emotion intensity scores]{
    Spearman's rank correlation coefficients between the valence/arousal scores and the emotion intensity scores across the seven evaluator conditions (HUMAN: using the average ratings from human evaluators; others: using scores from AI-based evaluators). 
    The abbreviations are as follows: DET/STO denote the determinism of the responses (Deterministic setting/Stochastic setting); GPT/CLD/GMN denote the language models (GPT/Claude/Gemini).
    To account for multiple comparisons, p-values were adjusted using the Benjamini–Hochberg correction procedure to control the false discovery rate within each evaluator condition. 
    Asterisks indicate statistical significance after the correction (*: $p < 0.05$, **: $p < 0.01$, ***: $p < 0.001$). 
    Blank entries indicate cases where the LLM responses collapsed, making the computation infeasible.
  }
  \label{fig:va_emotion_correlation}
\end{figure*}

\clearpage
\subsection{Supplementary Analysis 2: Personality Traits and Image Features}
Here, we conducted a supplementary analysis focusing on the human aesthetic evaluation based on the data reported in~\citep{washizu2025bodily}. 
Specifically, we examined whether differences in personality traits modulate the strength of responses to image features. 

\textbf{Method: }
Using the full set of 9192 samples of aesthetic evaluations performed by 511 human participants across multiple images, we tested the interaction between individual personality traits and image features in predicting aesthetic ratings (beauty). 
Specifically, we constructed multiple regression models in which the aesthetic rating for each image served as the dependent variable, and interaction terms between personality trait scores and image features were included as explanatory variables. 
As personality traits ($z$), we considered the Big Five traits, alexithymia tendencies, interoceptive awareness, empathy-related traits, sensitivity to beauty in nature, art, and morality, as well as self-reported physical condition on the day of the experiment. 
As image features ($x$), we included Composition, Light, Color, Depth of Field, Content, Content-Preference, and Willingness-To-Share. 
For each combination of personality trait and image feature, a separate regression model of the following form was constructed. 
\begin{align}
  r_{h_{ij}}
  &= \beta_0 + \beta_1\,x_{j} + \beta_2\,z_{i} + \beta_3\,(x_{j} z_{i}) + \alpha_i + \gamma_j + \varepsilon_{ij}
  \label{eq:interaction_model}
\end{align}
Here, $r_{h_{ij}}$ denotes the aesthetic rating assigned by human evaluator $i$ to image $j$, $z_i$ represents the personality trait of evaluator $i$, and $x_j$ denotes the image feature. 
The terms $\alpha_i$ and $\gamma_j$ represent fixed effects for the human evaluator and the image, respectively. 
Equation~\eqref{eq:interaction_model} was estimated for each combination of $x$ and $z$ using the least squares method. 
To account for within-evaluator correlation, robust standard errors clustered at the evaluator level were employed. 
Our primary interest lies in the significance of the interaction coefficient $\beta_3$ in the regression model.
To address multiple comparisons, p-values were adjusted using the Benjamini-Hochberg procedure, and those below 0.05 were considered statistically significant. 

\textbf{Results and Discussion: }
The results are shown in Figure~\ref{fig:interaction_heatmap}. 
From these results, significant interactions were observed between many personality traits and image features. 
This indicates that, depending on the level of a given personality trait, both the magnitude and direction of the effect of specific image features on the aesthetic rating $r_h$ can vary.
In other words, individual personality traits influence responsiveness to image features, suggesting that, when predicting individual aesthetic evaluations, it is necessary to adjust the importance of each image feature according to the personality traits of the individual.

\begin{figure}[H]%[ht]
  \centering
  \includegraphics[width=\columnwidth, trim=0 0 0 0, clip]{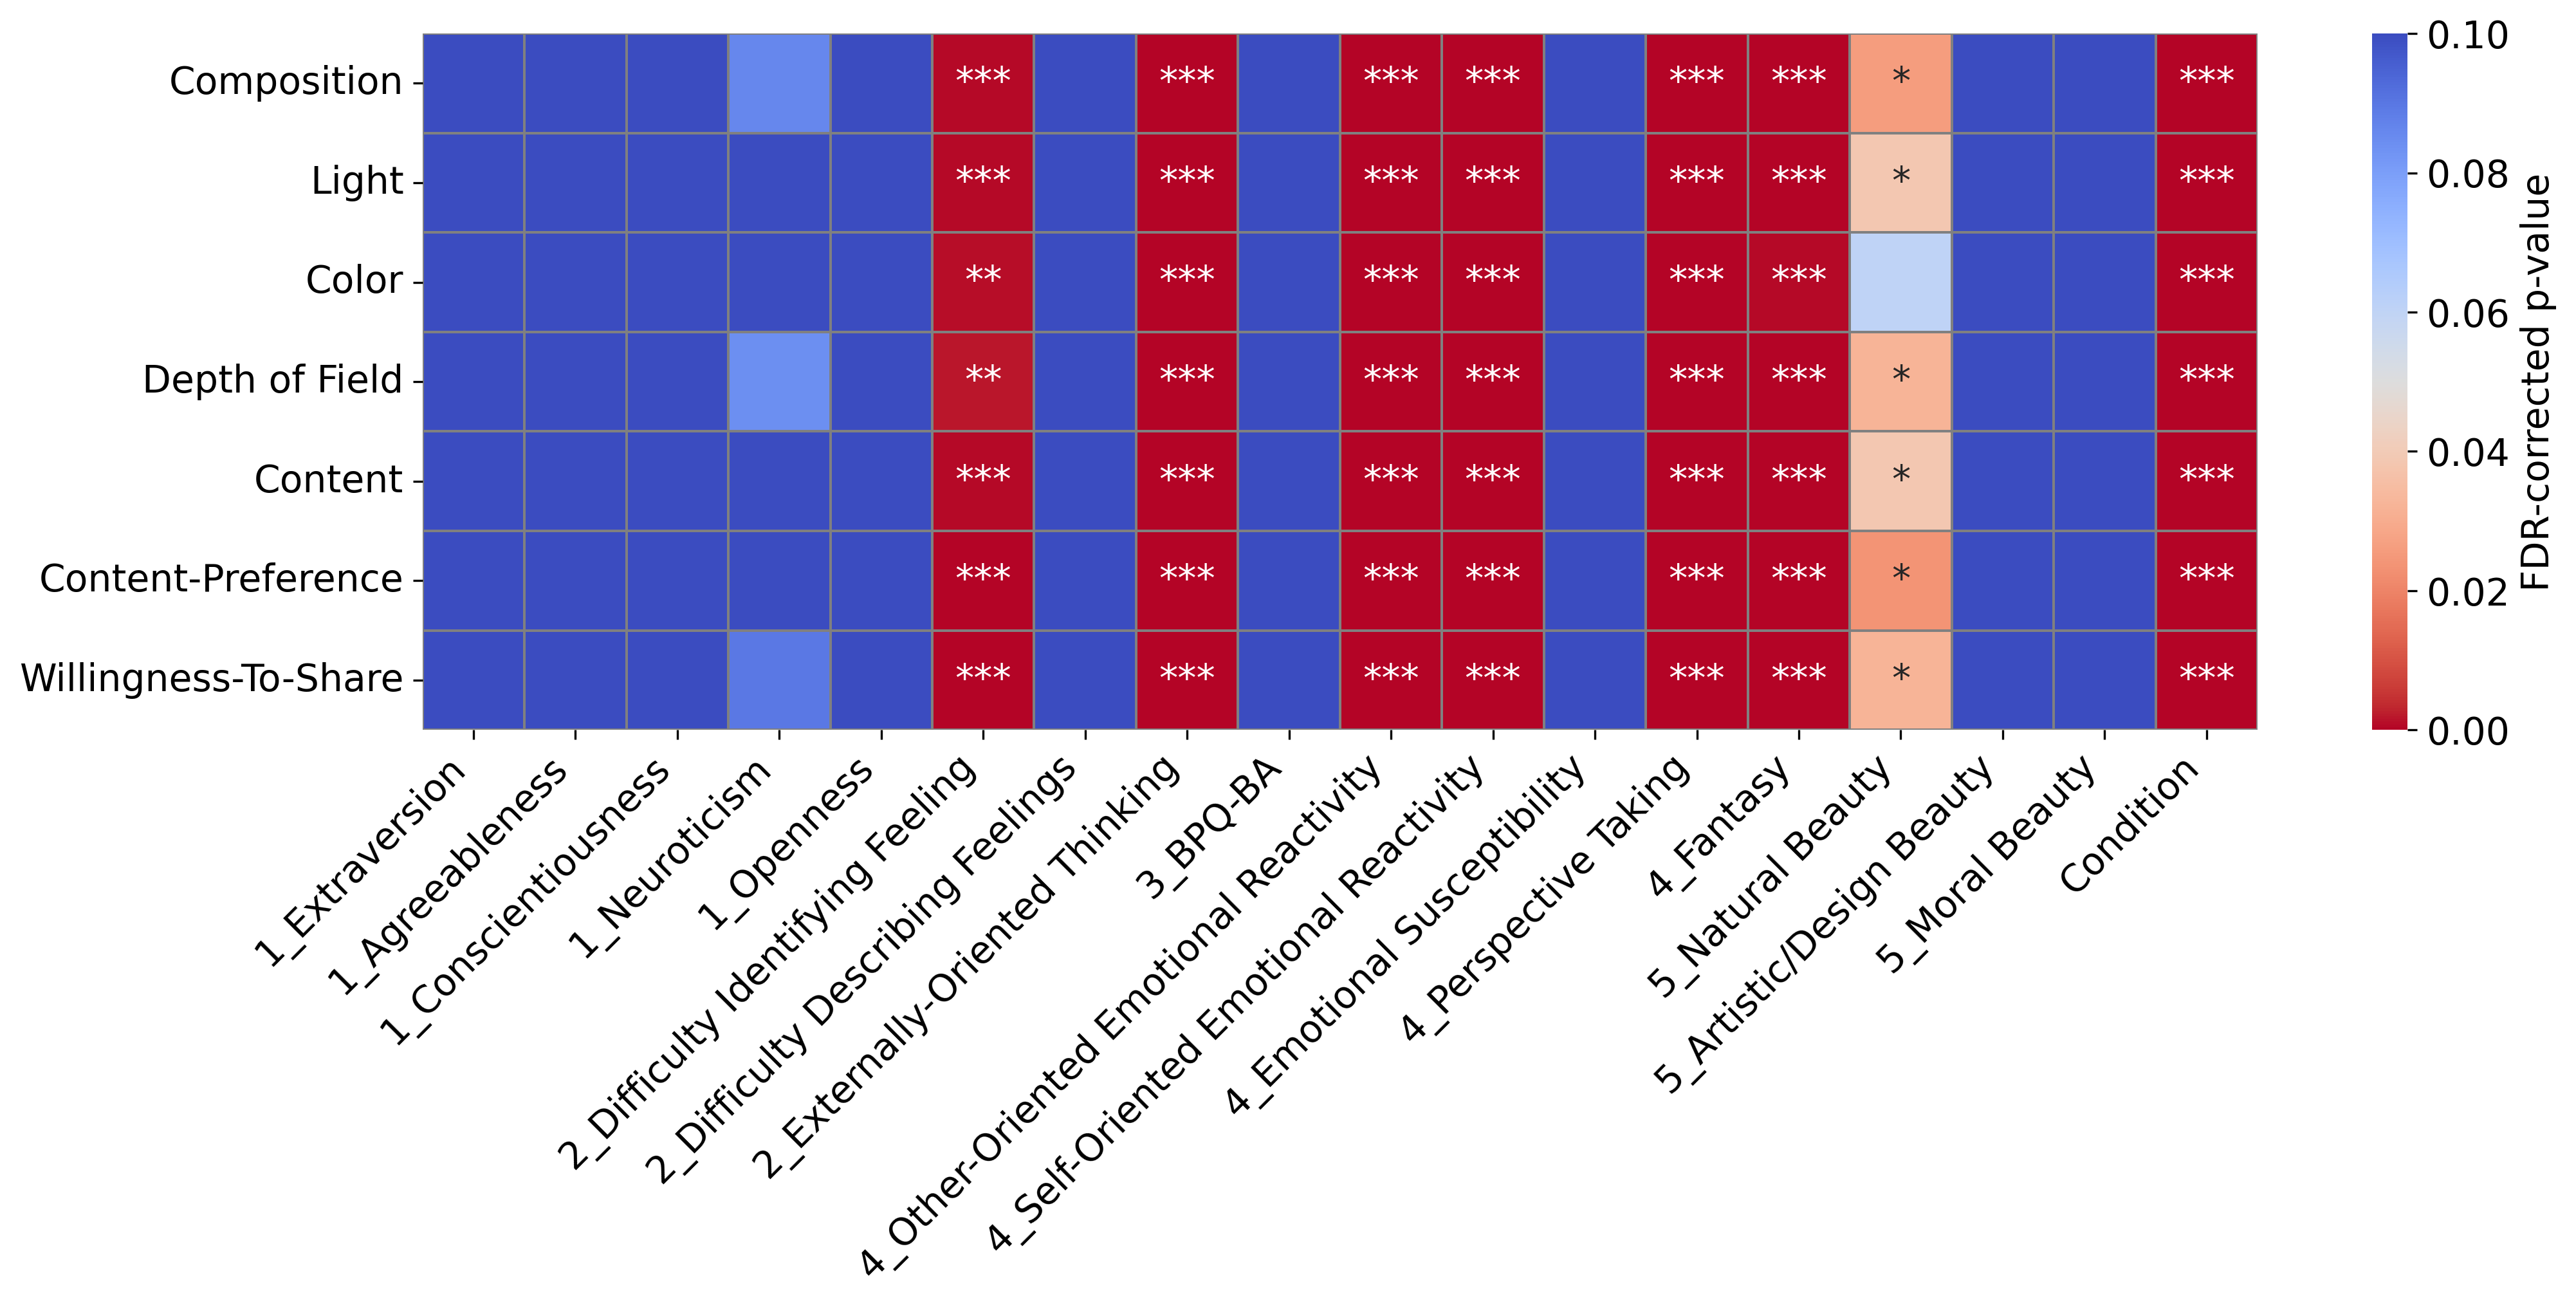}
  % \fbox{\rule{0pt}{4.5cm}\rule{0.98\columnwidth}{0pt}}
  \caption[Interaction between personality traits and image features]{
  Interaction between personality traits and image features with respect to the beauty score of individual human evaluators.
  To account for multiple comparisons, p-values were adjusted using the Benjamini-Hochberg correction procedure to control the false discovery rate. 
  Asterisks indicate statistical significance after the correction (*: $p < 0.05$, **: $p < 0.01$, ***: $p < 0.001$). 
  Cells display adjusted p-values for the interaction coefficient from separate regressions including the interaction between personality traits and image features.
  }
  \label{fig:interaction_heatmap}
\end{figure}

\clearpage
\subsection{Supplementary Analysis 3: Sad Beauty}
Here, we focused on the phenomenon of "sad beauty", in which sadness co-occurs with a sense of beauty. 

\textbf{Method: }
Images for which both the intensity of the Sadness emotion and the beauty score exceeded predefined thresholds were considered as exhibiting sad beauty. 
For the human response data, the ranking method was employed, in which only the top three emotion labels were reported and converted into non-negative intensity scores (see Analysis 1 for further details). 
Accordingly, a threshold of 0 was used, and images with a Sadness intensity score greater than 0 were classified as "sad" images. 
In contrast, beauty scores were reported on a 1-9 Likert scale; therefore, the mean and standard deviation across the 347 images were computed, and a threshold was defined as one standard deviation above the mean. 
That is, images with beauty scores exceeding the mean by more than one standard deviation were classified as "beautiful" images. 
Images satisfying both conditions (sadness and beauty) were defined as instances of sad beauty. 
Note that both the emotion intensity scores and beauty scores were averaged across multiple evaluators for each image. 

In contrast, for the AI response conditions, we adopted the rating method. 
Specifically, we used three models (GPT, Claude, and Gemini) under two determinism settings (deterministic and stochastic), resulting in a total of six conditions.
In this case, both emotion intensity scores and beauty scores were reported on a 1-9 Likert scale. 
Therefore, for both sadness and beauty, thresholds were defined as one standard deviation above the mean. 

\textbf{Results and Discussion: }
The distribution of the 347 images in the human response data is shown in Figure~\ref{fig:sad_beauty_human}. 
The regression line indicates that as the sadness score increases, the beauty score decreases, confirming a negative correlation between sadness and beauty. 
On the other hand, 13 out of the 347 images were classified as exhibiting sad beauty. 
Although this accounts for less than 5\% of all images, it confirms that there are indeed images for which both sadness and beauty are highly rated. 

The distribution of the 347 images in the AI response data is shown in Figure~\ref{fig:sad_beauty_ai}. 
While there is variation across LLMs (e.g., no sad beauty images were observed for Claude, whereas Gemini showed the largest number), it is nevertheless confirmed that, even in AI evaluations, there exist images for which both sadness and beauty are highly rated.

\begin{figure}[H]%[ht]
  \centering
  \includegraphics[width=0.75\columnwidth, trim=0 0 0 0, clip]{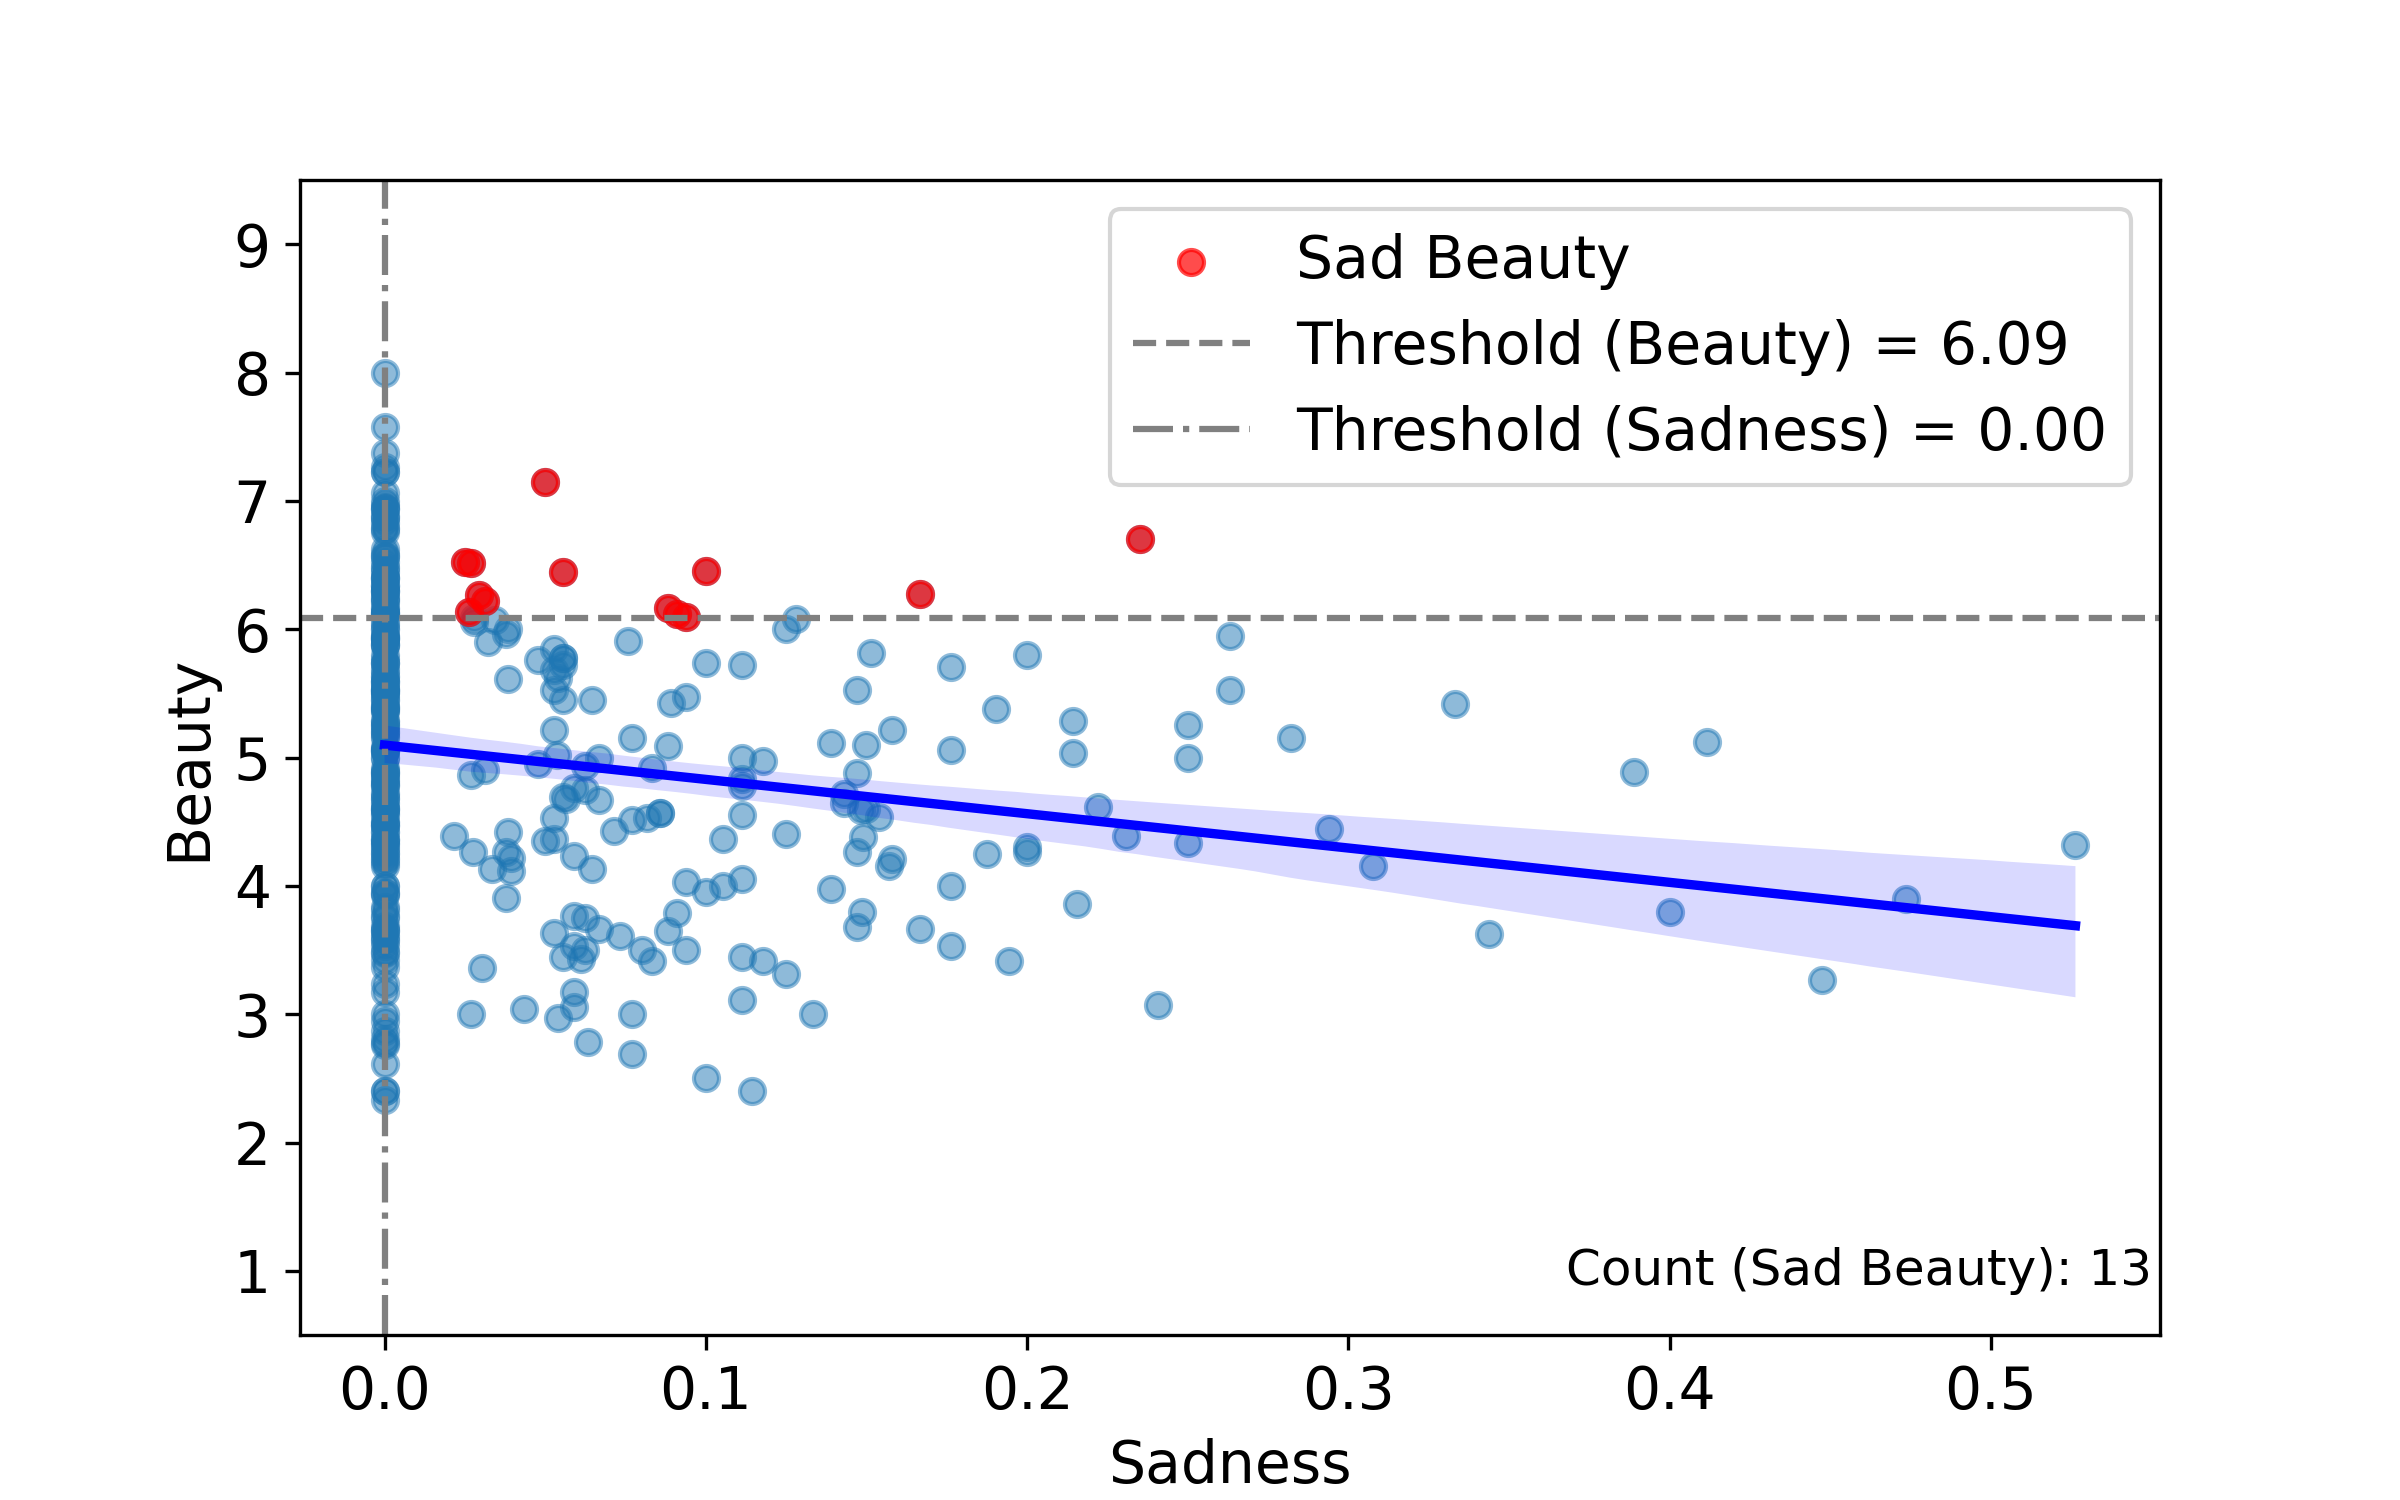}
  % \fbox{\rule{0pt}{4.5cm}\rule{0.98\columnwidth}{0pt}}
  \caption[Distribution of sadness and beauty scores (human evaluation)]{
    Distribution of sadness and beauty scores (human evaluation) across all 347 images. 
    Red dots indicate the images corresponding to sad beauty, with their total number shown in the lower right corner of the graph. 
    The blue line represents the regression line, and the shaded area indicates the 95\% confidence interval.
  }
  \label{fig:sad_beauty_human}
\end{figure}

\begin{figure}[H]%[ht]
  \centering
  \includegraphics[width=\columnwidth, trim=0 0 0 0, clip]{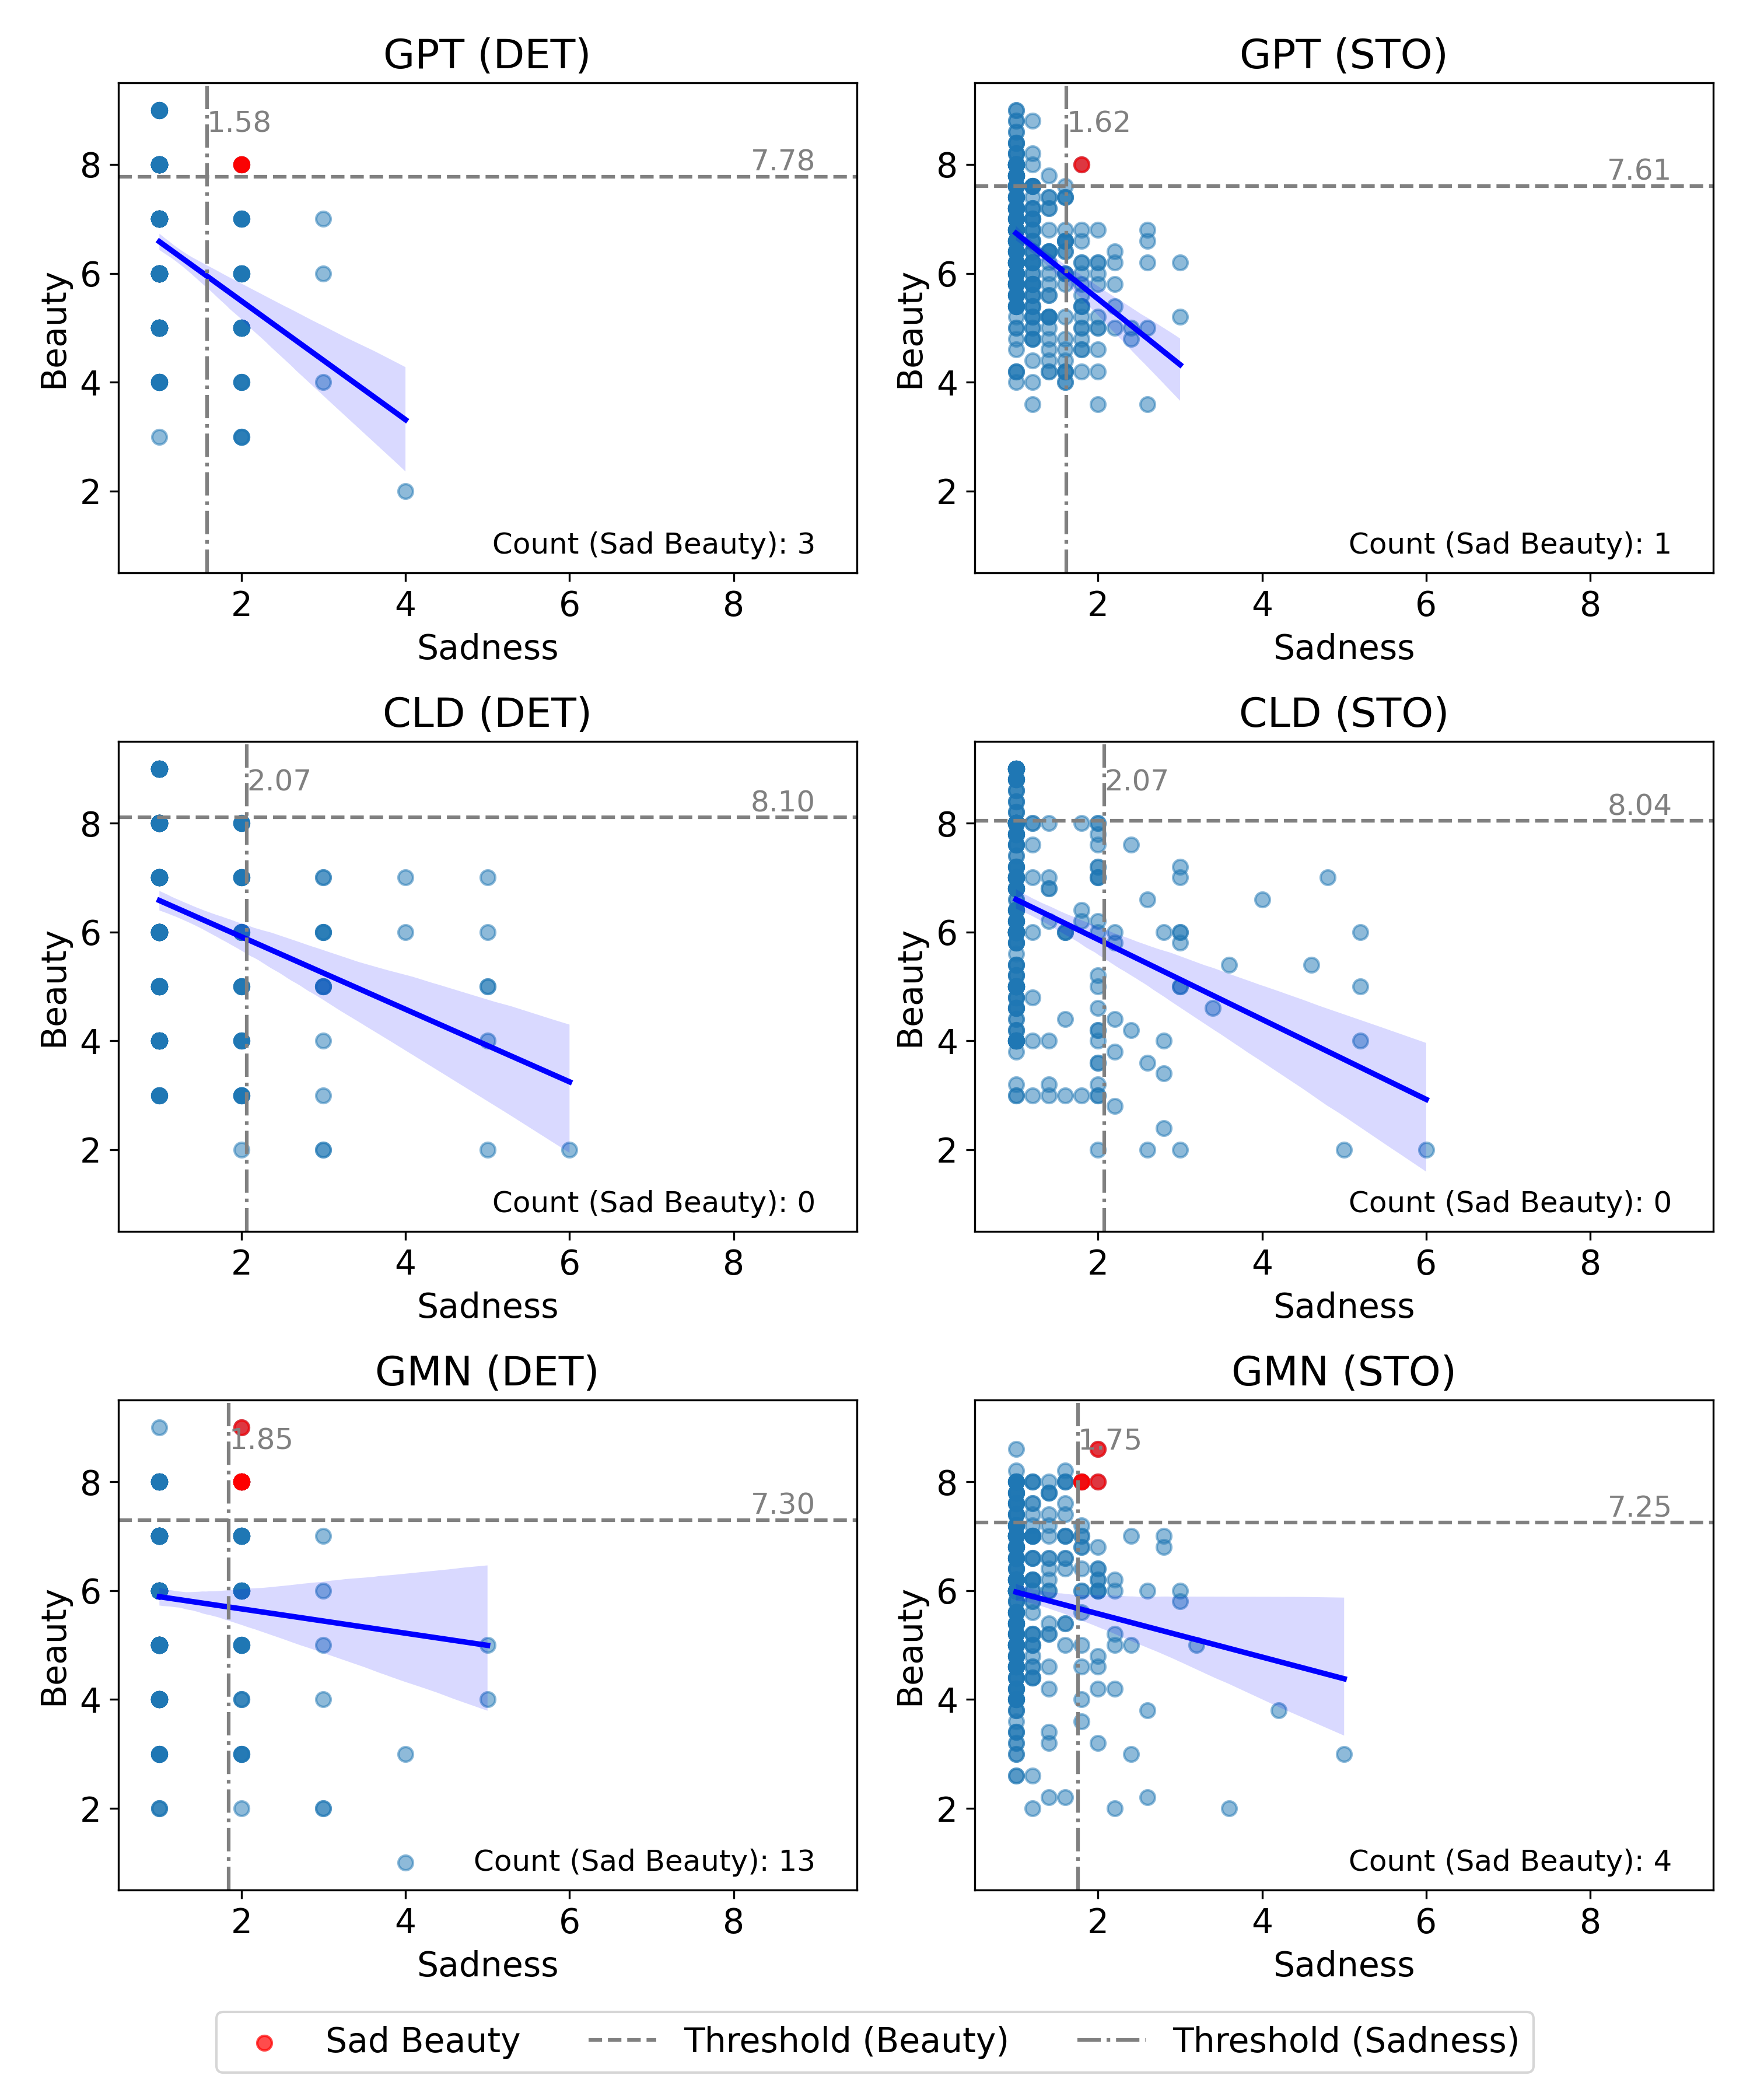}
  % \fbox{\rule{0pt}{4.5cm}\rule{0.98\columnwidth}{0pt}}
  \caption[Distribution of sadness and beauty scores (AI evaluation)]{
    Distribution of sadness and beauty scores (AI evaluation) across all 347 images. 
    Red dots indicate the images corresponding to sad beauty, with their total number shown in the lower right corner of each graph. 
    The blue line represents the regression line, and the shaded area indicates the 95\% confidence interval.
    The abbreviations are as follows: DET/STO denote the determinism of the responses (Deterministic setting/Stochastic setting); 
    GPT/CLD/GMN denote the language models (GPT/Claude/Gemini).
  }
  \label{fig:sad_beauty_ai}
\end{figure}
